# Supplementary material for: Robust linear-scaling optimization of compact localized orbitals in density functional theory
Source: arXiv:2004.05901 source file (2021-09-30)
Supplement: Supplementary file 1 [file SI.pdf]

# Supplementary Material for Robust linear-scaling optimization of compact localized orbitals in density functional theory

Yifei Shi, Jessica Karaguesian, and Rustam Z. Khaliullin*

*Department of Chemistry, McGill University,*

*801 Sherbrooke St. West, Montreal, QC H3A 0B8, Canada*

## RELATION BETWEEN THE HESSIAN AND PRECONDITIONER

The second derivative of the energy with respect to the CLMO coefficients is

$$\begin{aligned}
\Gamma_{\bar{x}\mu,\bar{y}\nu}{}^{xi,yj} &\equiv \frac{\partial^2 E}{\partial T^{\bar{y}\nu}{}_{yj} \partial T^{\bar{x}\mu}{}_{xi}} \\
&= 4\langle \chi_{\bar{x}\mu} | (\hat{I} - \hat{R}) \hat{H} (\hat{I} - \hat{R}) | \chi_{\bar{y}\nu} \rangle \sigma^{yj,xi} - \\
&- 4\langle \chi_{\bar{x}\mu} | (\hat{I} - \hat{R}) | \chi_{\bar{y}\nu} \rangle \langle \phi^{yj} | \hat{H} | \phi^{xi} \rangle - \\
&- 4\langle \chi_{\bar{x}\mu} | \phi^{yj} \rangle \langle \chi_{\bar{y}\nu} | (\hat{I} - \hat{R}) \hat{H} | \phi^{xi} \rangle - \\
&- 4\langle \chi_{\bar{x}\mu} | (\hat{I} - \hat{R}) \hat{H} | \phi^{yj} \rangle \langle \chi_{\bar{y}\nu} | \phi^{xi} \rangle - \\
&+ 4 \sum_{z,w} \langle \chi_{\bar{x}\mu} | (\hat{I} - \hat{R}) | \chi^{z\lambda} \rangle \frac{\partial \hat{H}_{z\lambda,w\kappa}}{\partial T^{\bar{y}\nu}{}_{yj}} \langle \chi^{w\kappa} | \phi^{xi} \rangle
\end{aligned}$$

The preconditioner defined in the main text is an approximation to this Hessian. The preconditioner is evaluated only within the same domain (i.e. $y = x$) and the $T$-dependence of the Kohn-Sham Hamiltonian is neglected (i.e. the last term is assumed to be zero). Additionally, the $\sigma^{xj,xi}$ is approximated with the identity matrix and $\langle \phi^{xj} | \hat{H} | \phi^{xi} \rangle$ is set to $-\delta_{ji}$. The third and fourth terms are also neglected because, for $x = y$, they contain the gradient, which becomes small as the ground state is approached in the iterative procedure.

## EIGENVALUES OF THE PRECONDITIONER

Figure S1 shows the eigenvalues of the preconditioner for several cases in a typical calculation. For completely delocalized orbitals, the eigenvalues are either exactly zero (occupied-occupied mixing) or very large (occupied-virtual mixing). For the straightforward optimization of CLMOs, the eigenvalue spectrum is continuous and low-curvature modes exist. For the optimization with the low-curvature projector (LCP) and $\Lambda_c = 0.02$ a.u., the small and large eigenvalues are again separated.

## PHYSICAL ORIGIN OF THE LOW-CURVATURE MODES

In the main text, we suggested that the low-curvature optimization modes represent occupied-hybrid mixing modes, where the hybrid states are mostly but not completely occupied. These occupied-hybrid modes directions exist in the vector space of domain $\bar{x}$ because CLMOs of the neighbor centers are not completely localized on $\bar{x}$. Our hypothesis implies that a hybrid low-curvature mode $|d_{\bar{x}p}\rangle$ has only small component in the unoccupied subspace of domain $\bar{x}$. This

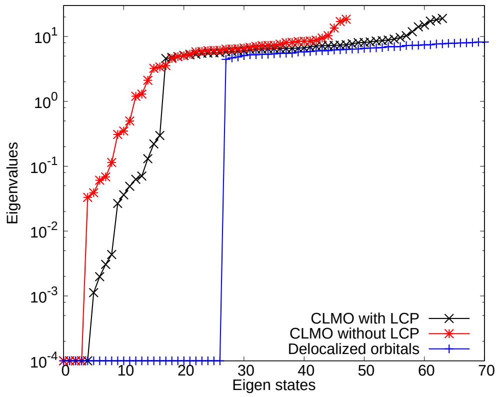


FIG. S1. Eigenvalues of the preconditioner in the final stages of the PBE/DZVP orbital optimization for hexagonal CdSe lattice with eight atoms. To display the zero eigenvalues on the logarithmic scale, all eigenvalues values are shifted up by $10^{-4}$ a.u. For the CLMO optimization, the localization domain includes the central $Cd^{2+}$ ion and three $Se^{2-}$ ions. For the delocalized orbitals, the domain includes the entire system and only low eigenvalues are shown. For the CLMO optimization without the low-curvature projector, the calculation does not converge and the preconditioner is evaluated at final iterations, for which the energy is close to the ground state.

component is measured by the residue $\Delta_{\bar{x}p}$

$$\Delta_{\bar{x}p} \equiv \langle d_{\bar{x}p}|\hat{I}_{\bar{x}} - \hat{R}_{\bar{x}}|d_{\bar{x}p}\rangle, \tag{S1}$$

where $\hat{R}_{\bar{x}}$ is a projector constructed from the occupied CLMOs of the neighbors truncated to the subspace $\bar{x}$ with operator $\hat{T}_{\bar{x}} \approx \hat{I}_{\bar{x}}$

$$\hat{R}_{\bar{x}} = \sum_{y,z\in\bar{x}} \hat{T}_{\bar{x}}|\psi_{yi}\rangle\sigma_{\bar{x}}^{yi,zj}\langle\psi_{zj}|\hat{T}_{\bar{x}} \tag{S2}$$

and $\sigma_{\bar{x}}$ is the overlap matrix of the truncated orbitals.

Unfortunately, it is difficult to unambiguously divide the vector space of a domain into the occupied $\hat{R}_{\bar{x}}$ and unoccupied $(\hat{I}_{\bar{x}} - \hat{R}_{\bar{x}})$ subspaces because of substantial electron delocalization between centers (i.e. atoms). In our definition, the unoccupied subspace is ultimately determined by what orbitals are included into projector $\hat{R}_{\bar{x}}$.

Here, we discuss the dependence of residues $\Delta$ on dimensionless parameter $t \in [0, 1]$ – a proxy for the tunable size of the *occupied* subspace of $\bar{x}$. First, we introduce a measure of what fraction of a normalized CLMO $|\psi_{yj}\rangle$ is present outside domain $\bar{x}$:

$$M_{yj}^{\bar{x}} \equiv \langle\psi_{yj}|(\hat{I} - \hat{I}_{\bar{x}})|\psi_{yj}\rangle \tag{S3}$$

Second, we include only those $|\psi_{yi}\rangle$ states into $\hat{R}_{\bar{x}}$ whose presence outside $\bar{x}$ is below

$$M_{yj}^{\bar{x}} < t \tag{S4}$$

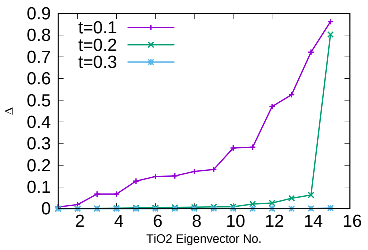


FIG. S2. $\Delta$ as a function of $t$ for $Ti^{4+}$ ions in the $TiO_2$ rutile lattice.

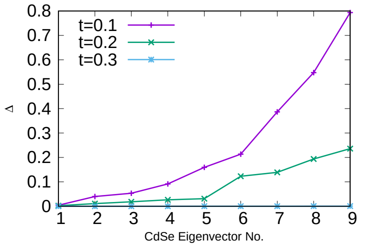


FIG. S3. $\Delta$ as a function of $t$ for $Cd^{2+}$ ions in the CdSe Wurtzite lattice.

where cutoff threshold $t \in [0, 1]$. For example, $t = 0.2$ means that $\hat{R}_{\bar{x}}$ includes the orbitals, whose presence on $\bar{x}$ is 80% or more. For larger $t$, more and more states outside $\bar{x}$ are included into $\hat{R}_{\bar{x}}$ thus reducing the dimension of the unoccupied space on $\bar{x}$ and, as a consequence, bringing $\Delta$ down.

The dependence of $\Delta$ on $t$ for the materials described in main-text is shown in Figures S2–S5. The assumption that the low-curvature modes have small presence in the unoccupied space holds for $TiO_2$, CdSe, water cluster with atomic partitioning. However, it is less accurate for Si where optimal CLMOs are less localized.

## DOGLEG TRUST REGION ALGORITHM

The LCP method, described in the main text, is essentially a regularized preconditioned conjugate gradient (PCG) algorithm. In the PCG algorithm, the search direction is determined first

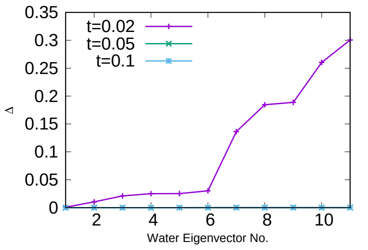


FIG. S4. $\Delta$ as a function of $t$ for $O^{2-}$ in water tetramer.

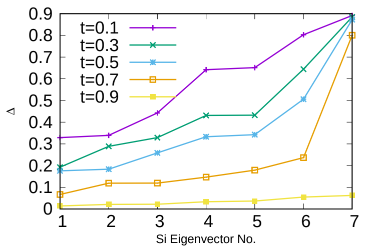


FIG. S5. $\Delta$ as a function of $t$ for Si atom in the diamond silicon lattice.

and then the loss function (i.e. the electronic energy in our case) is minimized along the chosen direction using a one-dimensional search algorithm.

Trust-region (TR) methods is another family of algorithms that are suited to deal with ill-conditioned problems with low-curvature modes. In contrast to the PCG algorithm, TR algorithms determine the search direction and one-dimensional step size simultaneously. At each TR iteration [1], the model quadratic subproblem is solved within the multidimensional sphere of a set *trust* radius to suggest an update to the current values of independent variables (matrix $\mathbf{T}$ in our case). If the updated loss function is similar to what was predicted from the quadratic model, the update is judged acceptable. Otherwise the independent variables remain unchanged and the trust radius is reduced to produce a new subproblem that is solved in the next iteration. There exist a variety of TR methods that differ by how the model function is defined and how the subproblem is solved. Here, the model quadratic function is expressed in terms of the exact analytical gradient and preconditioner given by Eqs. (6) and (7) in the main text, respectively. The dogleg algorithm is used to solve the subproblem [1].

Figure S6 shows the performance of the TR algorithm for the CMO optimization of the hexagonal CdSe – the system considered in detail in the main text. The TR algorithm does not result in significant improvement in the rate of convergence compared to the block-diagonal projector. The norm of the gradient does not decrease to the desired level. However, the energy decreases faster than with the block-diagonal projector. Nevertheless, the LCP optimizations with $\Lambda_c = 0.005$ a.u. and $\Lambda_c = 0.0005$ a.u. have significantly better rate of convergence in terms of both energy and the unprojected gradient than the TR algorithm. The analysis of the TR algorithm optimization reveals that the trust radius shrinks rapidly after several iterations (note the regions of $\Delta E = 0$ in the top panel where the trust radius is reduced), resulting in very ineffective optimization of the low curvature modes. This indicates that the model quadratic function does not reproduce the true energy function well. The cost of each iteration of the TR algorithm is noticeably higher than that of the LCP iteration because the Hessian has to be inverted in every iteration of the TR

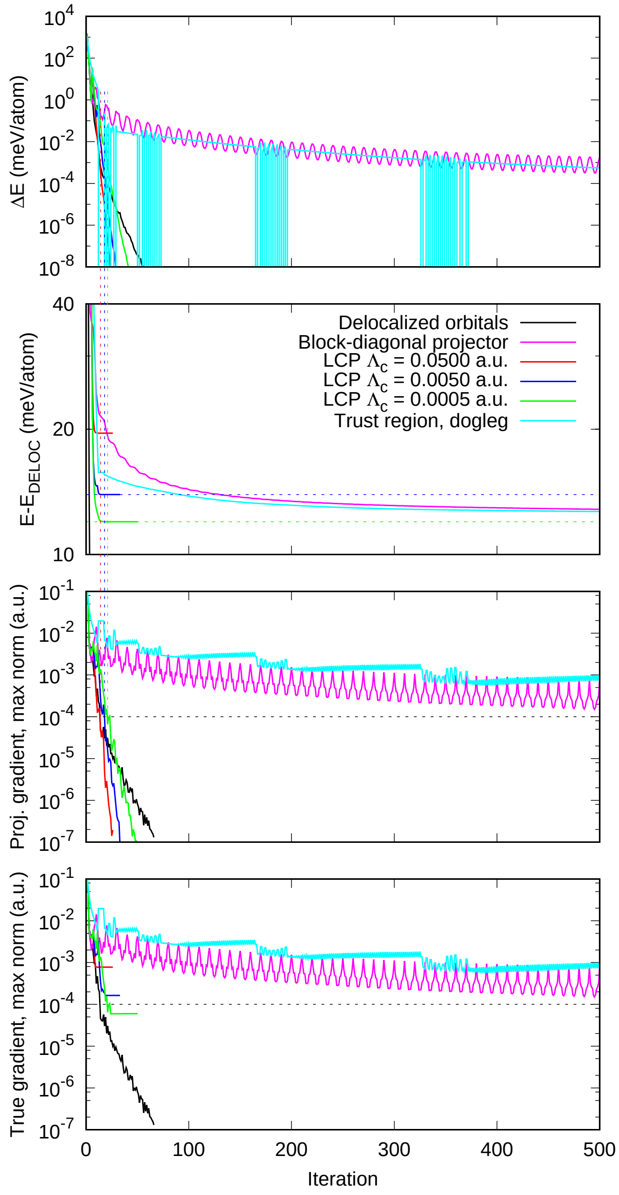


FIG. S6. Optimization of the CLMOs for the hexagonal wurtzite CdSe lattice. PBE/DZVP, $R_c = 4.9$ Å. In the top panel, the energy does not decrease ($\Delta E = 0$) when the trust radius in the TR algorithm is reduced.

method and only occasionally in the LCP method.

---

* rustam.khaliullin@mcgill.ca

[1] J. Nocedal and S. Wright, *Numerical Optimization* (Springer Science & Business Media, 2006).

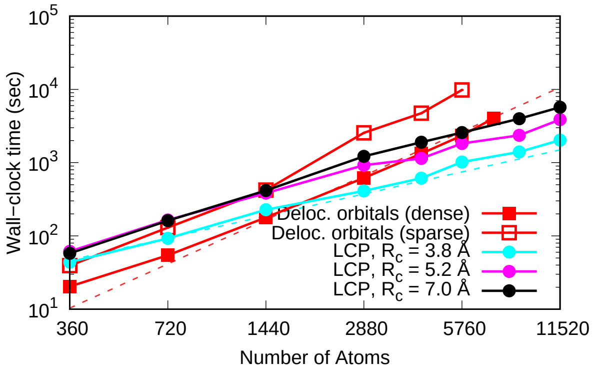


FIG. S7. Timing benchmark for the hexagonal phase of CdSe described at the PBE/DZVP level of theory on 400 compute cores. In LCP calculations, $\Lambda_c = 0.005$ a.u. Dashed lines show perfect linear and quadratic scaling. Note that with the employed settings, OT calculations cannot be performed due to the high memory demands of handling delocalized molecular orbitals.
